# Supplementary material for: Towards Smart Point-and-Shoot Photography
Source: arXiv:2505.03638 source file (2025-05-06)
Supplement: Supplementary file 1 [file X_suppl.tex]

\clearpage
\setcounter{page}{1}
\maketitlesupplementary

In this document, we provide more details as supplementary materials to our main submission. We first present the related work. We present the mathematical details of view generation from equirectangular panoramas to perspective views in our proposed Panorama-based Composition Adjustment Recommendation dataset (PCARD) in \cref{sec:PCARD}, followed by the definition and calculation of spherical overlap and spherical IoU metrics in \cref{sec:Sph}. In \cref{sec:statistics}, we provide comprehensive statistical information of our proposed PCARD, including its taxonomic structure and detailed label analysis. \cref{sec:ablation} presents extensive ablation studies on our CLIP-based Composition Quality Assessment (CCQA) model. Finally, in \cref{sec:subjective}, we describe our subjective evaluation setup and provide additional qualitative results demonstrating the effectiveness of our approach across diverse scenarios.

\section{Related Work}

The image cropping (ICDB) dataset \cite{ICDB} and the human crop (HCDB) dataset \cite{HCDB} contain a small number of images that were manually annotated with the best cropping boxes by multiple professional photographers. Since the best cropping generated in this manner relies entirely on the annotators' experience without explicit constraints, Christensen and Vartakavi \cite{GNMC} constructed an aspect ratio-aware image cropping (GNMC) dataset, where each image includes optimal cropping annotations in different aspect ratios (16:9, 3:4, 4:3, 2:2, 1:1).The subject-aware composition (SACD) dataset \cite{SACD} contains 2777 images and more than 24,000 candidate views, where each image is annotated with 8 optimal cropping boxes. However, the limited number of annotated crops is not conducive to the training of a robust image composition model. Therefore, some other datasets \cite{r1,r4,r5, r7,r10,SACD} were created with dense annotations. The primary paradigm of creating these datasets is first generating a large number of candidate views, followed by experts annotating them using a pair-wise ranking strategy \cite{r1,r4} or a direct scoring approach \cite{r5,r7,r10}. The flicker-cropping (FCDB) dataset \cite{r1} contains 1743 images and 31430 annotated pairs of candidate views while the comparative photo composition (CPC) dataset \cite{r4} contains 10800 images, with 24 candidate views for each image and generates more than 1 million view pairs. The labeled cropping windows all have high aesthetic value with a certain focused subject. Different from the pair-wise strategy, the grid-anchor-based image cropping (GAICv1, GAICv2) dataset \cite{r7,r5} provides an average of 86 fixed candidate views for each image, where each candidate view is assigned an aesthetic quality score. The user-generated content crop (UGCrop5K) dataset \cite{r10} consists of 45000 exhaustively annotated candidate views on 5K images.

\begin{table}[t]  
    \centering  
    \resizebox{1\columnwidth}{!}{  
    \begin{tabular}{cccccc}  
    \toprule  
    Dataset & Year & Label & Scenes & \makecell{Candidate\\ Views}  & \makecell{Camera \\Pose}  \\
    \hline  
    ICDB\cite{ICDB} & 2013 & Best & 950 & 1 & N/A \\
    HCDB\cite{HCDB} & 2014 & Best & 500 & 1 & N/A \\
    GNMC\cite{GNMC} & 2022 & Best & 10000 & 5 & N/A \\
    SACD\cite{SACD} & 2023 & Best & 2777 & 8  & N/A  \\
    \hline  
    FCDB\cite{r1} & 2017 & Rank & 1536 & 18 & N/A \\
    CPC\cite{r4} & 2018 & Rank & 10800 & 24 & N/A \\
    GAICv1\cite{r7} & 2019 & Score & 1236 & 86 & N/A \\
    GAICv2\cite{r5} & 2020 & Score & 3336 & 86 & N/A  \\
    UGCrop5K\cite{r10} & 2024 & Score & 5000 & 90 & N/A  \\
    \bottomrule  
    \end{tabular}}  
    \caption{Image Composition datasets.}  
    \label{tab:dataset}  
\end{table}

\section{View Generation}
\label{sec:PCARD}
\begin{figure}[t]
    \centering
    \includegraphics[width=0.99\linewidth]{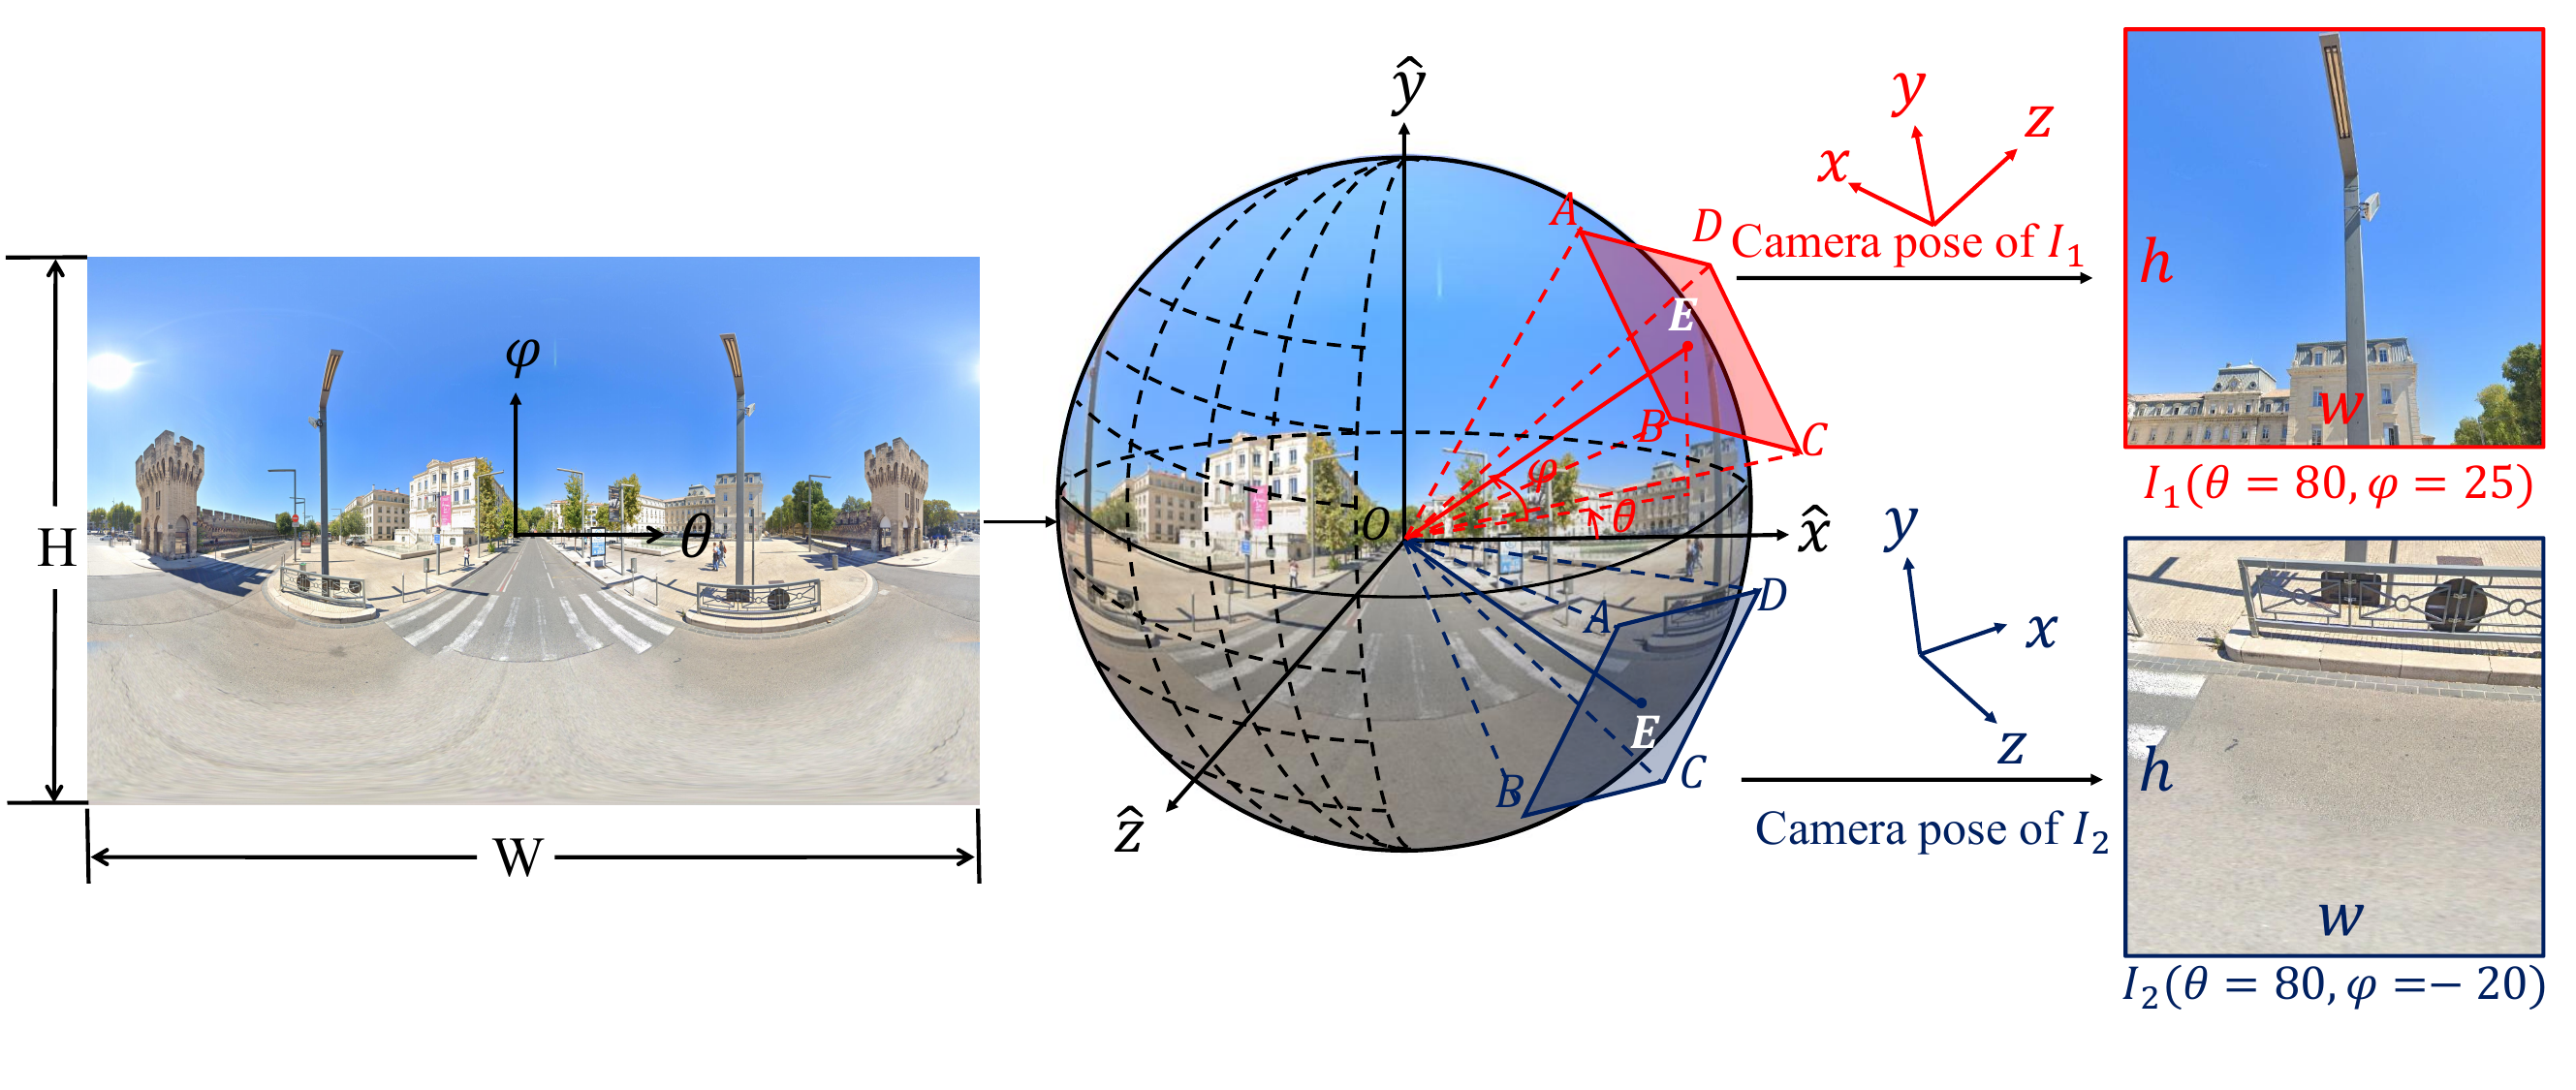}
    \caption{View generation. An equirectangular (ERP) image can be mapped to a perspective view using camera field of view ($fov_x, fov_y $) and viewing direction $(\theta_{0,0}, \varphi_{0,0})$ parameters.}
    \label{fig:4_perspective}
\end{figure}

\label{subsec:Data_Analysis}
\begin{figure*}[t]
    \centering
    \includegraphics[width=1\linewidth]{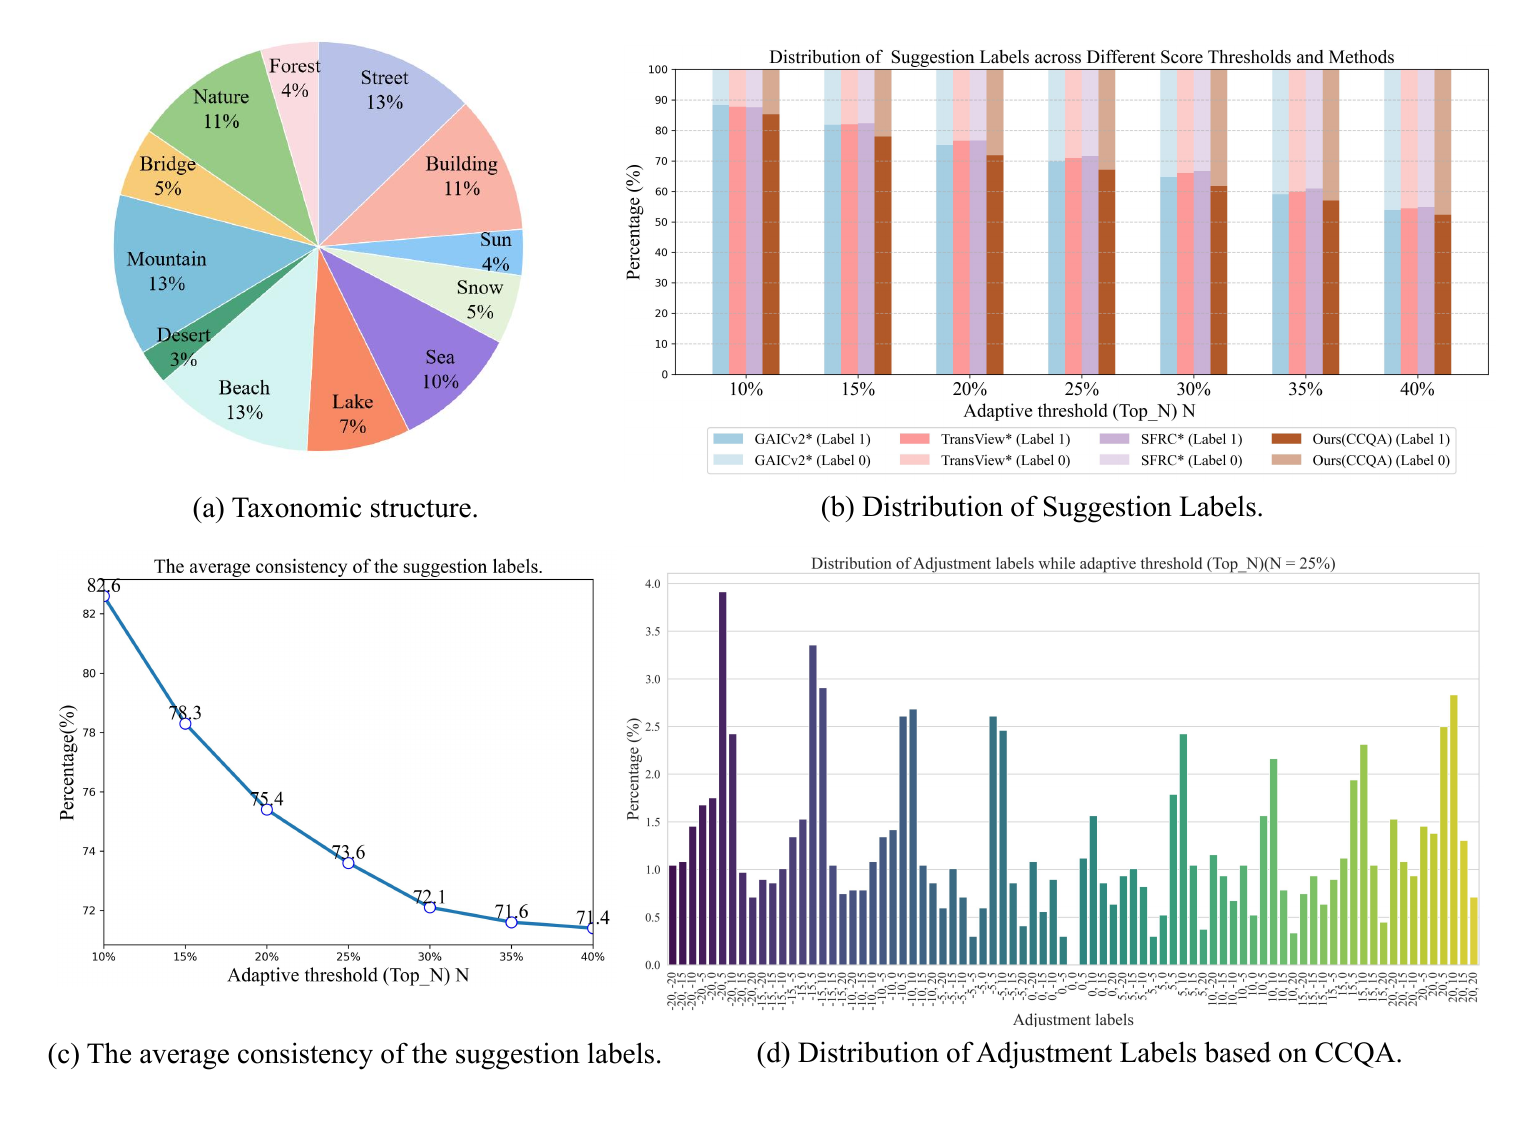}
    \caption{Statistics of the proposed PCARD dataset.}
    \label{fig:PCAR}
\end{figure*}

As shown in \Cref{fig:4_perspective}, we can generate a perspective view $I$ from an Equirectangular(ERP) image given two key parameters: (1) the camera field of view ($fov_x,fov_y$), and (2) the viewing direction $(\theta_{0,0}, \varphi_{0,0})$ that defines the viewpoint $E$ in the spherical domain $S^2$. The generated view $I$ has a spatial resolution of $h \times w$ in the 2D plane. Given a pixel located at ($i, j$) ($i\in[1,w], j\in[1,h]$) in the view $I$, we transform it into a 3D point $(x_{i, j}, y_{i, j}, z_{i, j})$ in the camera coordinate system through inverse perspective projection:
\begin{equation}
\left[\begin{array}{l}
x_{i, j} \\
y_{i, j} \\
z_{i, j}
\end{array}\right]=\left[\begin{array}{ccc}
f_x & 0 & i_0 \\
0 & f_y & j_0 \\
0 & 0 & 1
\end{array}\right]^{-1}\left[\begin{array}{l}
i \\
j \\
1
\end{array}\right]
\end{equation}
\begin{equation}
\left\{\begin{array}{l}
f_x=\frac{w}{2 \tan \left(\frac{f o v_x}{2}\right)} \\
f_y=\frac{h}{2 \tan \left(\frac{f o v_y}{2}\right)}
\end{array}\right.
\end{equation}
where $f_x$ and $f_y$ are the horizontal and the vertical focal lengths. Following \cite{zhu2021viewing}, we standardize all views with a vertical FOV of $fov_y = 60^{\circ}$ and a fixed spatial resolution of $h \times w = 768 \times 1024$. The principal point $(i_0, j_0)$ represents the pixel coordinates of the center point on the view $I$, where $i_0=(w-1)/2,j_0=(h-1)/2$.

To align the camera coordinate system $(x, y, z)$ with the world coordinate system $(\hat{x},\hat{y}, \hat{z})$, we apply two successive rotations:
\begin{equation}
\left[\begin{array}{l}
\hat{x}_{i, j} \\
\hat{y}_{i, j} \\
\hat{z}_{i, j}
\end{array}\right]=\mathcal{R}_y\left(\theta_{0,0}\right) \mathcal{R}_x\left(\varphi_{0,0}\right)
\left[\begin{array}{l}
x_{i,j} \\
y_{i,j} \\
z_{i,j} 
\end{array}\right]
\end{equation}
where $\mathcal{R}_y(\theta_{0,0})$ represents the rotation matrix of angle $\theta_{0,0}$ along $y$-axis, $\mathcal{R}_x(\varphi_{0,0})$ represents the rotation matrix of angle $\varphi_{0,0}$ along $x$-axis.
The rotated coordinates $(\hat{x}_{i,j},\hat{y}_{i,j}, \hat{z}_{i,j})$ are then converted to spherical coordinates (longitude $\theta_{i,j}$ and latitude $\varphi_{i,j}$ ):
\begin{equation}
\left\{\begin{array}{l}
\theta_{i,j}=\arctan \left(\frac{\hat{x}_{i, j}}{\hat{z}_{i, j}}\right) \\
\varphi_{i.j}=\arcsin \left({\hat{y}_{i, j}}\right)
\end{array}\right.
\end{equation}

Finally, we map these spherical coordinates to pixel coordinates $(u_{i,j},v_{i,j})$ in the ERP image domain with width $W$ and height $H$:
\begin{equation}
\left\{\begin{array}{l}
u_{i, j}=\left(\frac{\theta_{i, j}}{2 \pi}+\frac{1}{2}\right) W \\
v_{i, j}=\left(-\frac{\varphi_{i, j}}{\pi}+\frac{1}{2}\right) H
\end{array}\right.
\end{equation}

Through the series of coordinate transformations, we establish a complete mapping from the source ERP image to the target perspective view, enabling accurate view generation from any given viewpoint.

\section{Spherical overlap and Spherical IoU}
\label{sec:Sph}
Given a spherical rectangle $S_i(\theta_i, \varphi_i,\alpha_i,\beta_i)$, the area of the shape is $A(\cdot)$:
\begin{equation}
A\left(S_i\right)=4 \arccos \left(-\sin \frac{\alpha_i}{2} \sin \frac{\beta_i}{2}\right)-2 \pi \text {, for } i \in\{1,2\} 
\end{equation}
where ${\theta_i}$ and ${\varphi_i}$ denote the polar angle, $\alpha_i$ and $\beta_i$ represent the horizontal and vertical field of view. 
The overlapping region between two spherical rectangles is most likely not a standard spherical rectangle but rather an irregular spherical polygon, making the calculation of Area $A(S_i \cap S_j)$ quite complex. However, we can utilize the fact that the boundaries of the two spherical rectangles are great circle arcs and can be used to calculate the area of the overlapping region \cite{xu2022pandora}:
\begin{equation}
A\left(S_i \cap S_j\right)=\sum_{i=1}^n \omega_i-(n-2) \pi 
\end{equation}
where $n$ is the number of sides of the spherical polygon defined by the intersection region, $\omega_i$ is the angle of the spherical polygon, which is the angle between the planes on the adjacent boundaries.

Therefore,
\begin{equation}
\text{ SphOverlap }\left(S_{\text {adj }}, S_{\text {init}}\right)=\frac{A(S_{\text {adj }} \cap S_{\text {init }})}{A(S_{\text {init }})}
\end{equation}
\begin{equation}
\text{ SphIoU }\left(S_{\text {adj}}, S_{\text {init}}\right)=\frac{A(S_{\text {adj }} \cap S_{\text {init}})}{A(S_{\text {adj }}) + A(S_{\text {adj }}) -A(S_{\text {adj }} \cap S_{\text {init}})}
\end{equation}
where ${S}_{adj}$ and ${S}_{init}$ represent the spherical rectangles corresponding to $\boldsymbol{I}_{{adj}}^{i}$ and $\boldsymbol{I}_{{init}}^{i}$ in the $360^{\circ}$ images respectively.

\section{Statistics of the PACRD}
\label{sec:statistics}
\textbf{Taxonomic structure}. To better explore the aesthetic diversity of the PCARD, we manually divided it into 12 categories, namely Street, Building, Sun, Snow, Sea, Lake, Beach, Desert, Mountain, Bridge, Nature, and Forest, as shown in \Cref{fig:PCAR} (a). It is worth noting that, unlike common image composition datasets with single semantic information, these categories are not mutually exclusive, as individual images may contain multiple semantic elements. This is because the images in PCARD have richer semantic information, with overlaps between categories.

\begin{table}[t]
\resizebox{1\columnwidth}{!}{ 
\begin{tabular}{c|ccc|cccc}  
\toprule 
No. & WS & FMR & LP &  $\overline{A c c_5}$ & $\overline{A c c_{10}}$ & $\overline{A c c_{5}^w}$ & $\overline{A c c_{10}^w}$ \\
\hline  
1 & \checkmark  &            &            & 49.4 & 65.5 & 34.7 & 49.2 \\
2 &             & \checkmark &            & 48.3 & 64.7 & 34 & 43 \\
3 & \checkmark  & \checkmark &            & 49.4 & 65.8 & 35 & 49.4 \\
4 & \checkmark  &            & \checkmark & 51.5 & 68 & 36.4 & 51.5 \\
5 &             & \checkmark & \checkmark & 50.4 & 66.7 & 35.7 & 50.3 \\
6 & \checkmark  & \checkmark & \checkmark & \textbf{56.1} & \textbf{72.6} & \textbf{39.8} & \textbf{55.5} \\
\bottomrule 
\end{tabular}}
\caption{Ablation study of different components in CCQA. “LP”, “FMR”, and “WS” are short for Learnable prompt, Feature mixers and regression, and Weighted summation respectively.}
\label{tab:CCQA_ablation}
\end{table}

\begin{table}[t]
\centering
\begin{tabular}{c|ccc|cccc}  
\toprule 
No. & $\mathcal{L}_{1}$ & $\mathcal{L}_{2}$ & $\mathcal{L}_{3}$ &  $\overline{A c c_5}$ & $\overline{A c c_{10}}$ & $\overline{A c c_{5}^w}$ & $\overline{A c c_{10}^w}$ \\
\hline  
1 & \checkmark  &            &            & 34.8 & 56.6 & 23.1 & 39.1\\
2 &             & \checkmark &            & 45.5 & 63.8 & 30.1 & 46.1 \\
3 & \checkmark  &            & \checkmark & 41.1 & 60.2 & 27.5 & 43.1 \\
4 &             & \checkmark & \checkmark & 50.1 & 68.5 & 33.7 & 50.7 \\
5 & \checkmark  & \checkmark &            & 48.8 & 65.4 & 34.3 & 50.7 \\
6 & \checkmark  & \checkmark & \checkmark & \textbf{56.1} & \textbf{72.6} & \textbf{39.8} & \textbf{55.5} \\
\bottomrule 
\end{tabular}
\caption{Ablation study of different loss functions in CCQA.}
\label{tab:CCQA_loss}
\end{table}

\textbf{Label analysis}. First, to evaluate the reliability and consistency of our pseudo-labeling method, we conducted the comparative analysis using four composition scoring models: our proposed CCQA model and three representative models (GAICv2*~\cite{r7}, TransView*~\cite{r8}, and SFRC*~\cite{r6})\footnote{*Exclude the RoDAlign branch for a fair comparison.} following the main paper. These models were selected for their diverse technical approaches, ranging from RoIAlign and RoDAlign feature fusion, visual elements dependencies modeling to spatial-aware feature and transductive learning. We then analyzed the distribution of the suggested labels $\boldsymbol{y}_{{s}}^{i}$ generated by these four composition scoring models under the pseudo-labeling method based on different score thresholds. The visualization results are shown in \Cref{fig:PCAR} (b). It can be observed that if the score thresholds are set consistently, the distributions of the suggested labels generated based on different scoring models exhibit similar patterns, indicating the stability of our pseudo-labeling approach. Furthermore, we calculated the consistency of suggestion labels generated by CCQA and three other models, as shown in \Cref{fig:PCAR} (c). The average consistency of suggestion labels reaches over $70\%$. This high level of agreement among different models demonstrates both the robustness of our proposed pseudo-label generation method and the reliability of labels generated based on the CCQA model. In particular, considering both the balanced distribution and average consistency of suggestion labels, we chose $N=25\%$ in practice. \Cref{fig:PCAR} (d) show the distribution of adjustment labels $\boldsymbol{y}_{{a}}^{i}$ based on CCQA while $N=25\%$. If the composition can be improved, the distribution of adjustment labels aligns with the eight-neighborhood candidate adjustment space defined by the dataset with a step size of $\Delta\theta = \Delta\varphi = 5^{\circ}$, indicating that our proposed pseudo-label generation method and CCQA model can be reasonably applied to generate adjustment labels without missing potential adjustment spaces.

\section{Ablation study of the CCQA}
\label{sec:ablation}
To comprehensively evaluate our proposed CLIP-based Composition Quality Assessment model (CCQA) and demonstrate the reliability of the scoring order in our PCARD dataset, we conduct extensive ablation studies to analyze the contribution of each component and loss function. The experiments are performed by training on the GAICv2 dataset \cite{r5} and testing generalization on the unseen CPC dataset \cite{r4}.

\textbf{Model architecture}.We first investigate the impact of different architectural components in CCQA. As shown in \Cref{tab:CCQA_ablation}, we systematically evaluate three key components: Learnable prompt (LP), Feature mixers and regression (FMR), and Weighted summation (WS). The baseline model with only FMR achieves $\overline{Acc_5}$ of $48.3 \%$, $\overline{Acc_{10}}$ of $64.7\%$, $\overline{A c c_{5}^w}$ of $34 \%$ and $\overline{A c c_{10}^w}$ of $43 \%$. Adding WS (No.1) or combining it with FMR (No.3) shows incremental improvements. The introduction of Learnable prompt (LP) significantly enhances performance, particularly when combined with other components. The full model incorporating all three components (No.6) achieves the best performance across all metrics, with $\overline{Acc_5}$ of $56.1\%$, $\overline{Acc_{10}}$ of $72.6\%$, $\overline{A c c_{5}^w}$ of $39.8\%$ and $\overline{A c c_{10}^w}$ of $55.5\%$ on unseen data.

\textbf{Loss function}. We further examine the effectiveness of our loss function design, particularly focusing on the intermediate feature constraint $\mathcal{L}_{3}$. As shown in \Cref{tab:CCQA_loss}, we compare our complete CCQA model with a variant without the $\mathcal{L}_{3}$ loss term. The baseline CCQA without $\mathcal{L}_{3}$ achieves $\overline{Acc_5}$ of $48.8\%$, $\overline{Acc_{10}}$ of $65.4\%$, $\overline{A c c_{5}^w}$ of $34.3\%$ and $\overline{A c c_{10}^w}$ of $49\%$ on unseen data. By incorporating $\mathcal{L}_{3}$, our complete model shows substantial improvements across all metrics. These results demonstrate that constraining intermediate features through $\mathcal{L}_{3}$ is crucial for improving the generalization capability of CCQA.

\begin{figure}[t]
    \centering
    \includegraphics[width=1\linewidth]{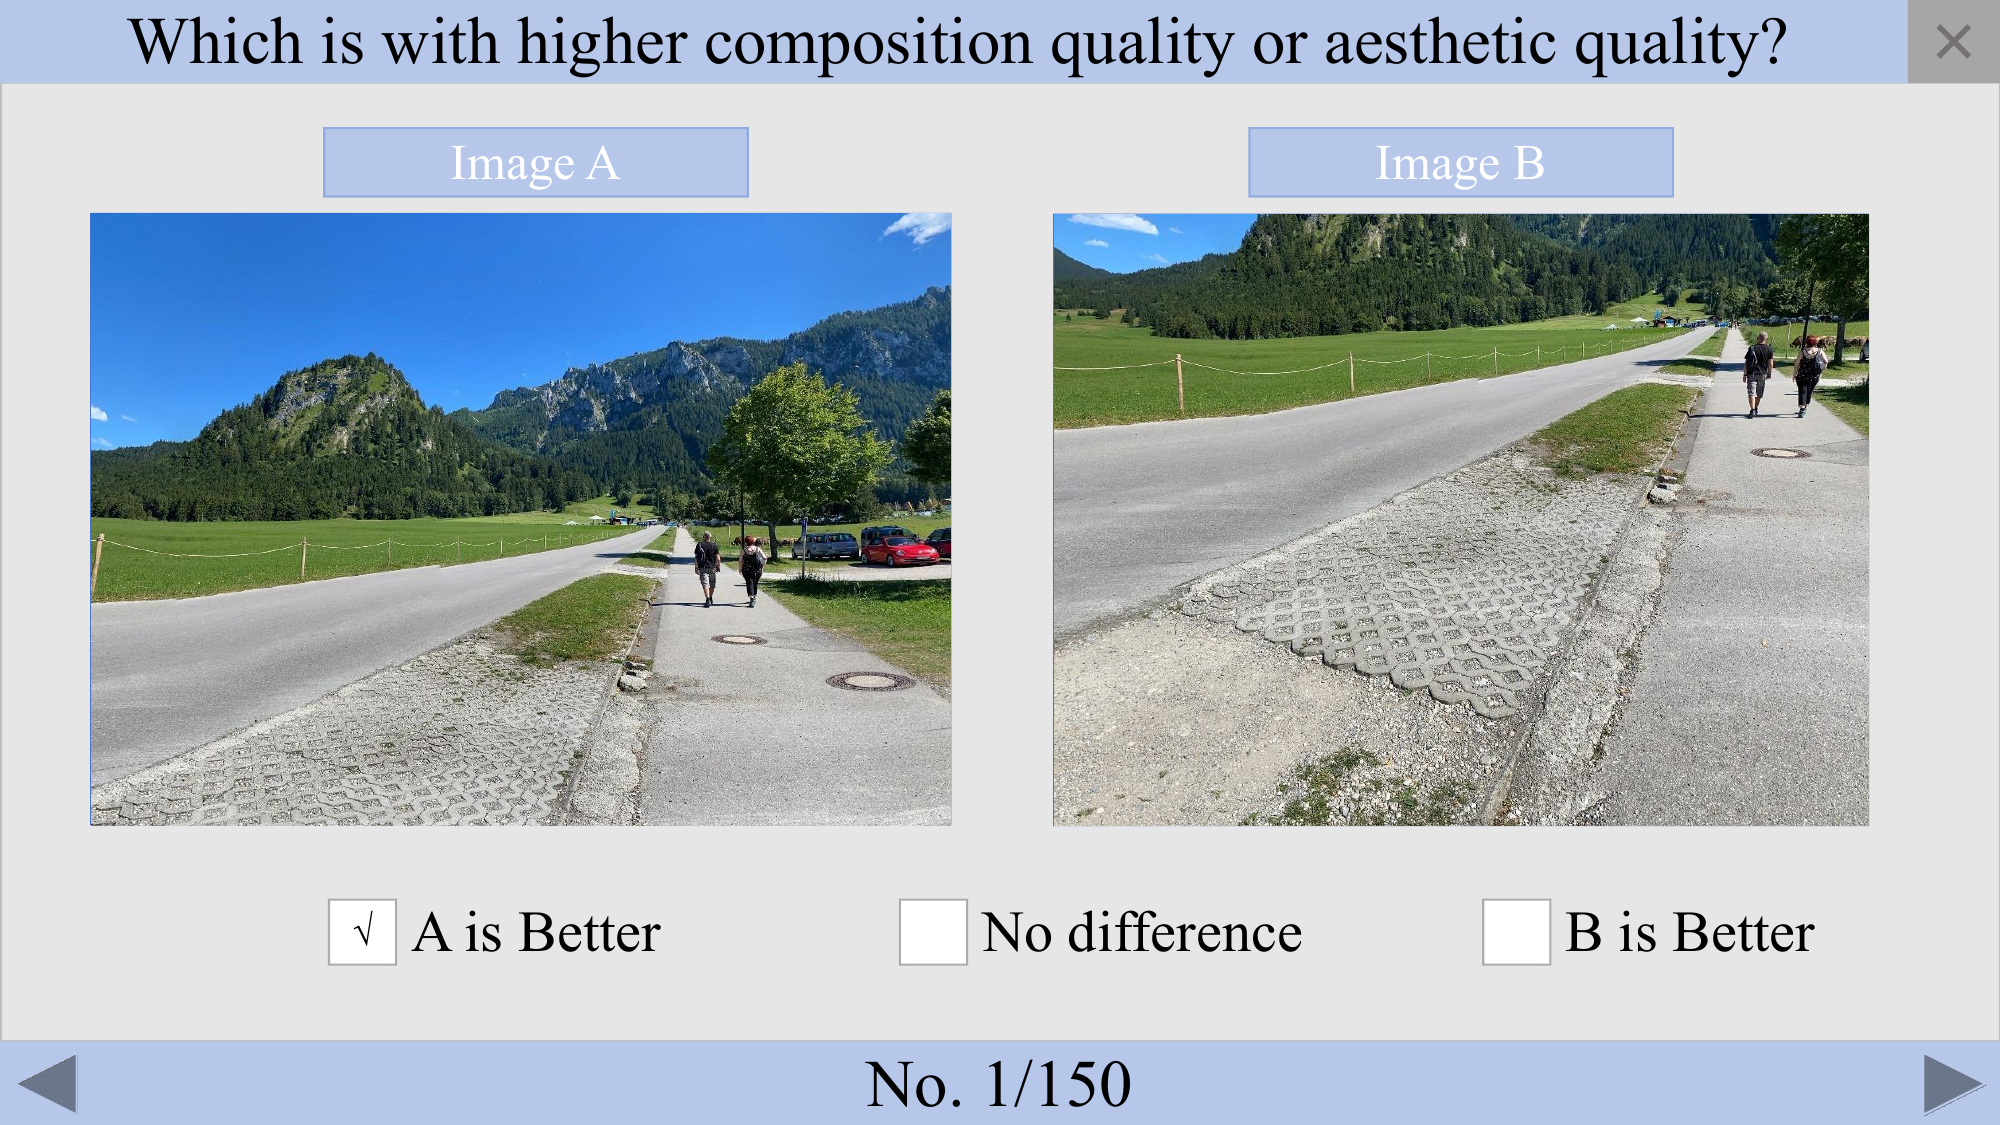}
    \caption{Illustration of the annotation toolbox.}
    \label{fig:userstudy}
\end{figure}

\section{Subjective Evaluation}
\label{sec:subjective}
\subsection{Annotation box}
The interface of our annotation toolbox for user studies is shown in \Cref{fig:userstudy}. The annotation toolbox was specifically designed to facilitate efficient and unbiased comparison of image compositions. The tool presents two images side-by-side for direct comparison, ensuring consistent evaluation conditions across all participants.
\begin{figure}[t]
    \centering
    \begin{subfigure}{0.2\textwidth}
        \centering
        \includegraphics[width=\textwidth]{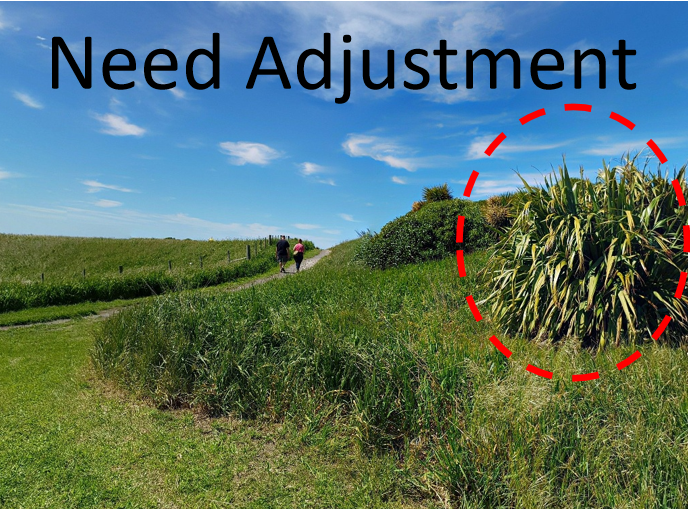}
    \end{subfigure}
    \begin{subfigure}{0.2\textwidth}
        \centering
        \includegraphics[width=\textwidth]{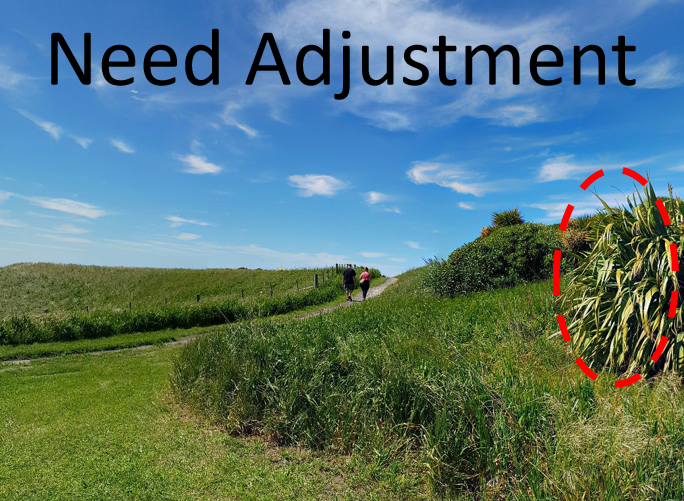}
    \end{subfigure}
    \begin{subfigure}{0.2\textwidth}
        \centering
        \includegraphics[width=\textwidth]{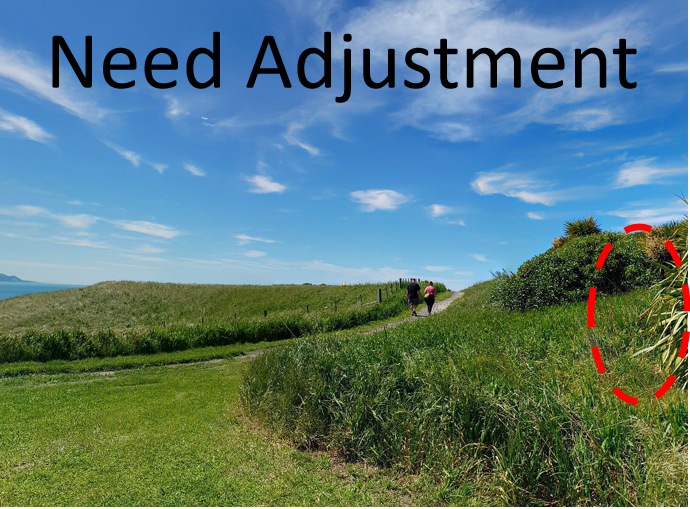}
    \end{subfigure}
    \begin{subfigure}{0.2\textwidth}
        \centering
        \includegraphics[width=\textwidth]{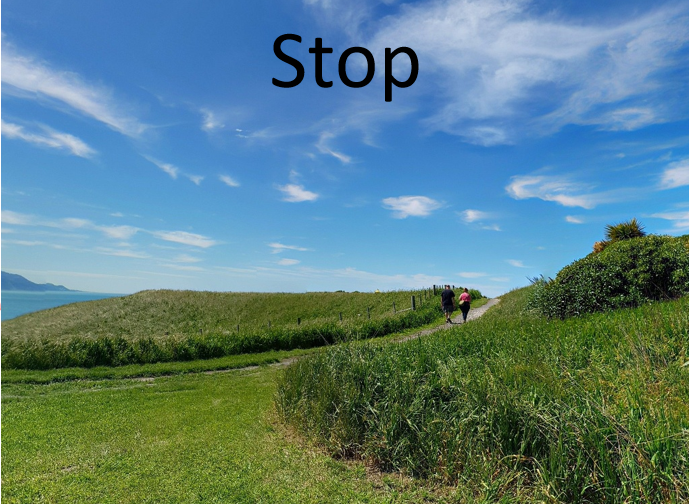}
    \end{subfigure}
     \caption{Examples of composition improvement trajectory: 3 steps. %From letf to right: initial view, intermediate adjustment, and final photograph 
    }
    \label{fig:qualitative_example1}
\end{figure}

\begin{figure}[t]
    \centering  
    \begin{subfigure}{0.15\textwidth}
        \centering
        \includegraphics[width=\textwidth]{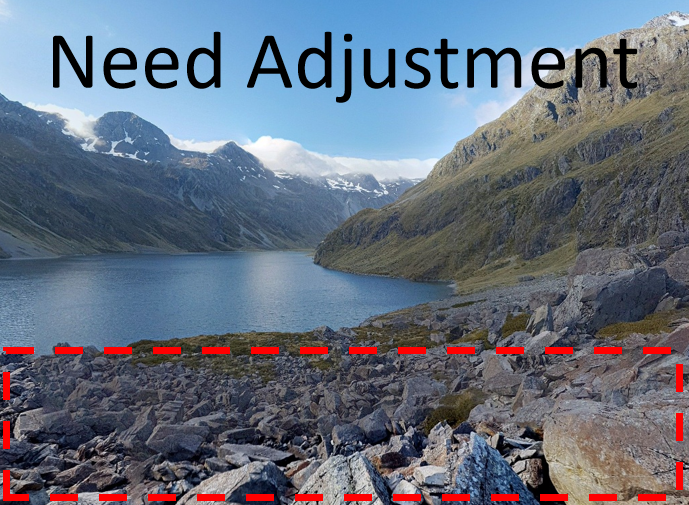}
    \end{subfigure}
    \begin{subfigure}{0.15\textwidth}
        \centering
        \includegraphics[width=\textwidth]{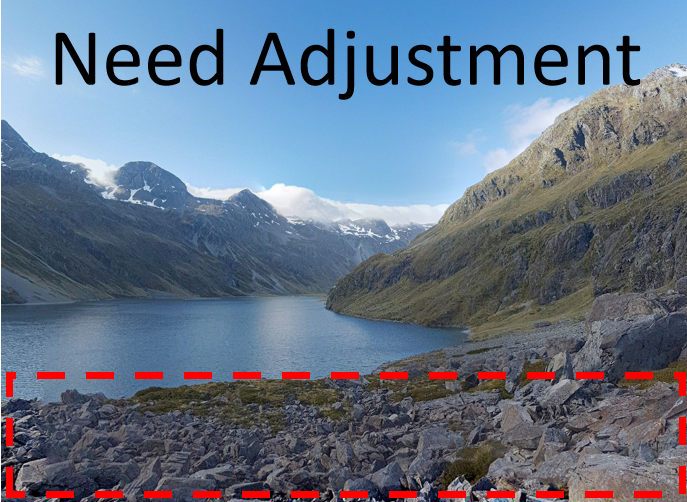}
    \end{subfigure}
    \begin{subfigure}{0.15\textwidth}
        \centering
        \includegraphics[width=\textwidth]{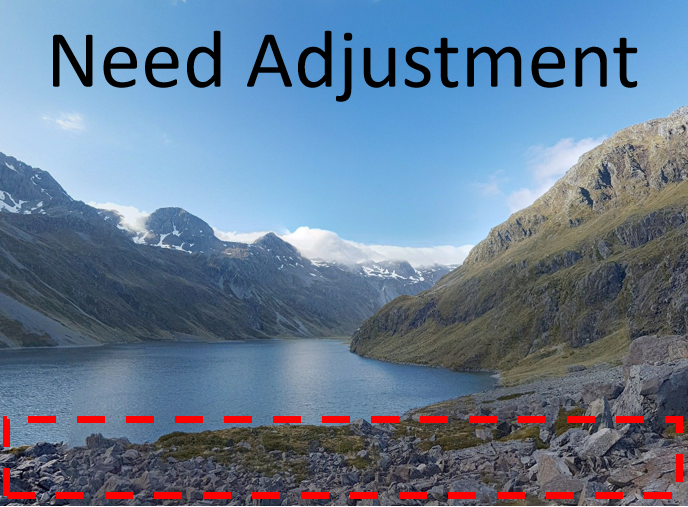}
    \end{subfigure}
    \begin{subfigure}{0.15\textwidth}
        \centering
        \includegraphics[width=\textwidth]{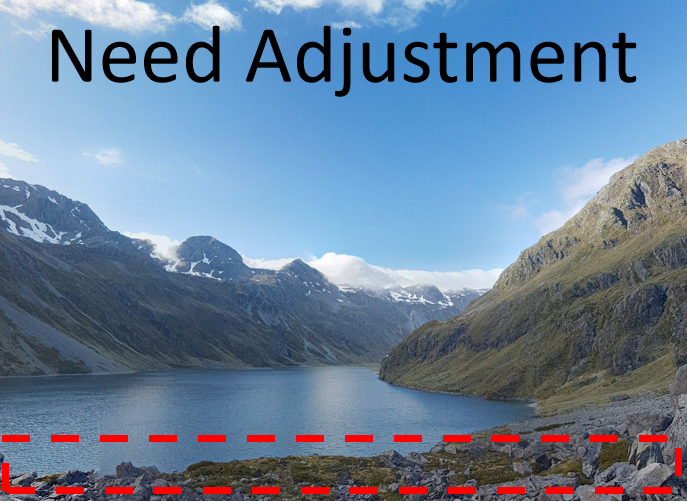}
    \end{subfigure}
    \begin{subfigure}{0.15\textwidth}
        \centering
        \includegraphics[width=\textwidth]{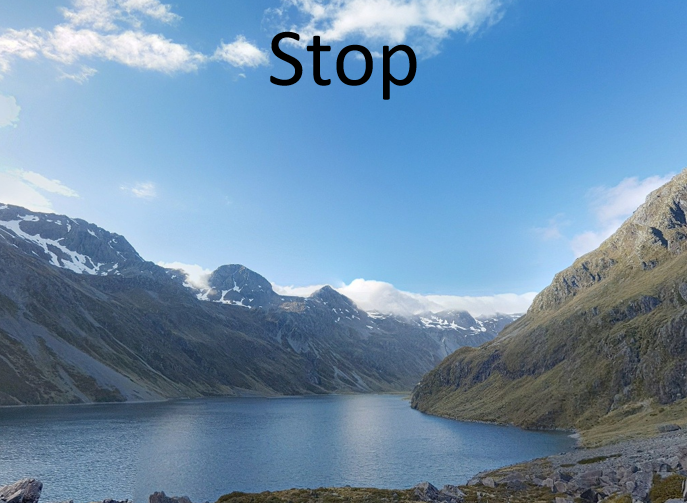}
    \end{subfigure}
  
    \caption{Examples of composition improvement trajectory: 4 steps. %From letf to right: initial view, intermediate adjustment, and final photograph 
    }
    \label{fig:qualitative_example2}
   
\end{figure}

\subsection{More qualitative results}
\begin{figure}[t]
    \centering
    \includegraphics[width=1\linewidth]{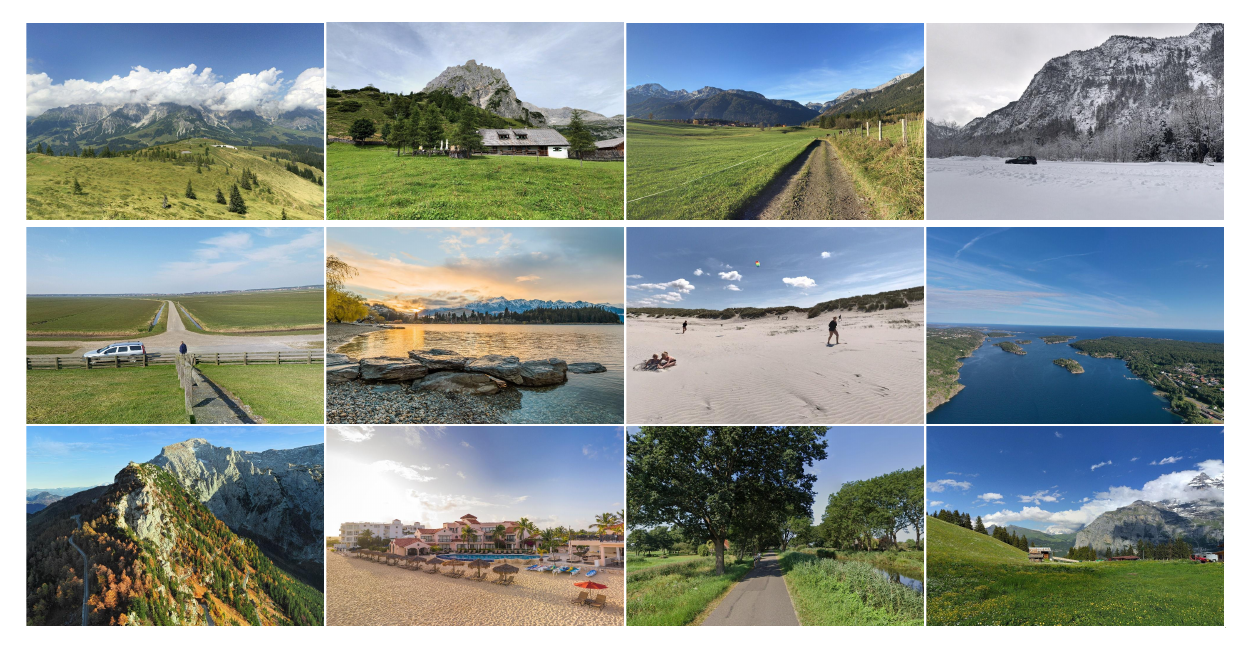}
    \caption{Examples of well-composed images requiring no adjustment.}
    \label{fig:suppl_no_need_adjust}
\end{figure}
\begin{figure*}[t]
    \centering
    \includegraphics[width=1\linewidth,keepaspectratio]{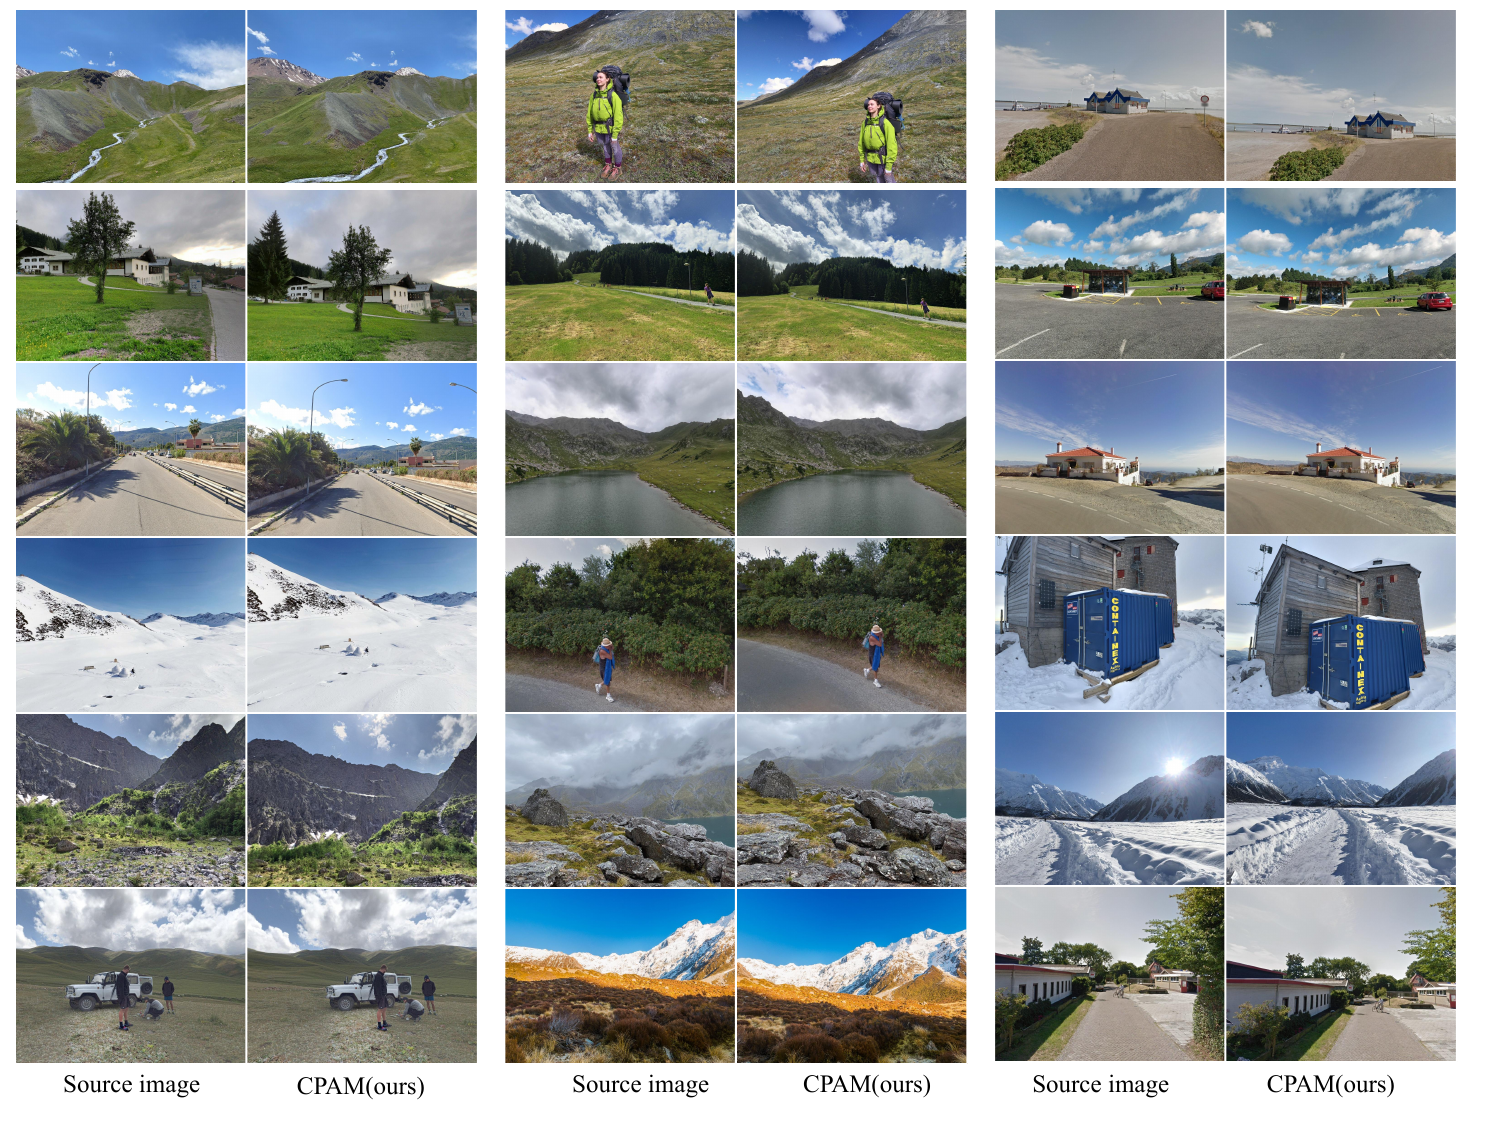}
    \caption{Demonstration of CPAM's adjustment capabilities: Before-and-after comparison on images requiring composition optimization.}
    \label{fig:suppl_subject}
\end{figure*}
This section shows more qualitative results. 

The sequence of operation of SPAS is as follows:
(i) Decide if the current composition can be improved by performing the suggestion prediction. (ii) If the suggestion predictor outputs 0, then the user will take a photo and the process is complete. (iii) If the suggestion predictor outputs 1, the system predicts the adjustment angles and the user follows the instruction to adjust the camera pose. (iv) Go to (i) and the process continues.Depending on the scene and initial view, it takes different number of steps, typically 3 to 6 in our data. \Cref{fig:qualitative_example1} and \Cref{fig:qualitative_example2} show examples of typical trajectories of improvement. 

To comprehensively evaluate our CPAM model's performance, we present two sets of qualitative results that demonstrate its intelligent decision-making capabilities across different scenarios. As shown in \Cref{fig:suppl_no_need_adjust}, we show cases where the source compositions are already well-crafted. These images, spanning various scenes including coastal landscapes, mountain views, and rural paths. \Cref{fig:suppl_subject} presents paired examples of images requiring compositional improvements, along with CPAM's adjustment results. Each pair consists of the source image and our model's optimized view. The adjustments demonstrate CPAM's effectiveness in various challenging scenarios: reframing landscapes to better emphasize focal points, optimizing horizon placement in outdoor scenes, and improving the balance of architectural elements. Notably, the adjustments are subtle yet meaningful, showing CPAM's ability to make refined modifications while preserving the essential character of each scene.These results collectively highlight CPAM's dual capability: maintaining already-optimal compositions while making appropriate adjustments when needed. This discriminative behavior is crucial for practical applications, where Smart Point-and-Shoot (SPAS) systems must be both effective and judicious in their interventions. The diverse range of scenarios in both figures also demonstrates the model's robust generalization across different photographic contexts and composition challenges.
